# Supplementary material for: Closing the Gap: A User Study on the Real-world Usefulness of AI-powered Vulnerability Detection & Repair in the IDE
Source: arXiv:2412.14306 source file (2025-04-25)
Supplement: Supplementary file 1 [file appendix.tex]

\section{Detection model}

We implemented our detection model (which we call \toolDetect{}) by fine-tuning CodeBERT~\cite{codebert}, following the procedure and using the dataset introduced in \citet{edittime}. We chose this model because it is suited to Edit-Time vulnerability detection, localization, and bug-type prediction, while other state-of-the-art models we considered~\cite{linevul,deepdfa} are trained on and primarily intended for complete code snippets without the ability to both localize lines and predict a specific bug type.
We fine-tuned \toolDetect{} for \textit{multi-task prediction}. For each given code snippet, it predicts: (1) whether the snippet contains a vulnerability, (2) whether any specific tokens in the snippet contain a vulnerability, and (3) the type of the vulnerability.
\Cref{fig:models-overview} shows an overview of our detection model approach. We replaced the final classifier layer (normally performing binary classification) with a layer of size ($d + k$), where $d$ is the number of tokens in the context window (512 for CodeBERT) and $k$ is the number of bug types in our training dataset (27 in our case), followed by a softmax layer. During training, we labeled the tokens (\ben{where did we get the ground-truth for labeling the tokens?}) with 1 when the code contained a vulnerability related to that token and 0 otherwise, did likewise for the bug types, and trained the model to jointly predict these $512 + 27 = 539$ classes for each example.
To train the model, we used a dataset collected using the same methodology as \citet{edittime}, consisting of vulnerable code snippets in public
GitHub repositories detected by CodeQL.

We trained \toolDetect{} on a dataset containing XXX code snippets in seven languages (C/C++, C\#, Go, Java, JavaScript/TypeScript, Python, and Ruby), including bug types corresponding to 27 CodeQL rules marked as impactful in the CWE database~\cite{cwe-database}, including Path Injection, SQL injection, Cross-Site Scripting (XSS), URL Redirection, Hard-coded Credentials, and Plain-Text Logging of Sensitive Data.
% \ben{TODO: Describe the dataset collection or say we re-used the dataset from the prior paper.}
We found that this multi-task fine-tuning was effective for providing localization and bug type classification, allowing the model to attain XXX loss and XXX validation accuracy during training.

\ben{Summarize and move to appendix.}
\wei{{\bf GPT filtering}}
During our experiments, we found that \toolDetect{} tended to make several cases of spurious predictions on certain bugs such as hard-coded credentials, plain-text logging of sensitive data, and SQL injection. These represent cases where correct detection requires nuanced decisions about the involved code and identifier names and may benefit from the emergent capabilities and greater capacity of large language models (LLMs) which might not be available for small language models (SLMs) similar to the scale of CodeBERT.
We also found that LLMs predicted more conservatively than fine-tuned SLMs, resulting in higher precision but lower recall \ben{Needs experimental support}.
% , often generating responses along the lines of ``As a large language model, I do not have enough information...''
However, many capable LLMs contain billions of parameters~\cite{scaling-laws} (compared to 125 million for our fine-tuned CodeBERT model~\cite{codebert}) and the closed-source weights cannot be optimized for production, which introduces latency which is unacceptable for scanning large corpora of source code; scalability was identified as a pain point for static analysis tools \cite{johnson_whydont_2013,christakis_whatdeveloperswantandneed_2016} \ben{TODO: check citation}.
To leverage the complementary benefits of both approaches, we used \toolDetect{} to detect potential vulnerabilities, then used an LLM to filter all vulnerable predictions.
We found that the LLM filter improved the precision by up to 20\% (see \Cref{sec:benchmarking}).

\begin{figure}[htbp]
    \centering
    \caption{The prompt used by \toolFix{}.}
\begin{minted}
[
framesep=2mm,
baselinestretch=1.2,
bgcolor=LightGray,
fontsize=\footnotesize,
breaklines
]
{python}
'''
A static analyzer has identified a {rule_id} security vulnerability in the {language} method below:

```
{method}
```

The SARIF result message is as follows: {message}

{description}

Write a fixed version of the method above and wrap it in triple backticks, then explain why your version addresses the problem.
'''
\end{minted}
    \label{fig:fix-prompt}
\end{figure}

We implemented our fix model (\toolFix{}) using GPT-4~\cite{gpt4} with specialized prompts shown in \Cref{fig:fix-prompt}. We chose this model because of its demonstrated high performance for generating bug-fixes and natural-language explanations, and the flexibility and generalization of LLM prompting approaches compared to fine-tuning \ben{Any citation available?}.
We prompted the model with instructions and the context surrounding the vulnerability alert; if the alert appears inside a function, we provide the entire function, and if it appears in a class or file, we provide the entire file.
